# Supplementary material for: The transience and persistence of high optical polarization state in beamed radio quasars
Source: arXiv:2301.06159 source file (2023-01-15)
Supplement: Supplementary file 1 [file online_materials_Blinov_Nov18.pdf]

Table 1: The basic optical data and the polarization classifications for the present sample of 83 radio quasars.

| Source<br>SDSS name<br>(1) | class<br>(2) | $z$<br>(3) | App. mag.<br>(SIMBAD)<br>B<br>V<br>R<br>(4) | App. mag.<br>(SDSS)<br>g<br>r<br>(5) | $p_{opt}$<br>(%)<br>(6) | Pol.<br>class<br>(7) | Epoch<br>(8) | $p_{opt}$ (%)<br>RoboPol<br>$p1$ (JD*)<br>$p2$ (JD*)<br>$p3$ (JD*)<br>mean $p$<br>(9) | N<br>(10) | Pol.<br>class<br>(RoboPol)<br>(11) |
|---|---|---|---|---|---|---|---|---|---|---|
| 0003-066<br>J000613.89-062335.33 | BZB | 0.347<br>0.347 | 19.10<br>—<br>17.14 | <br>18.56<br>17.87 | 1.4 ± 1.2 [F88]<br>**3.5 ± 1.6** [F88]<br>3.5 ± 1.0 [K90] | (HPQ) | 1984<br>1984<br>1987 | 34.4 ± 0.9 (6599)<br>26.1 ± 1.7 (6878)<br>25.3 ± 0.8 (6872)<br>< 21.20 > | 15 | HPQ |
| 0014+813<br>J001708.48+813508.14 | BZQ | 3.366<br>3.366 | 17.60<br>16.52<br>15.95 | <br>—<br>— | 1.1 ± 0.1 [K83] | LPRQ | 1982 | 1.8 ± 0.5 (6942)<br>1.0 ± 0.4 (7333)<br>0.5 ± 0.5 (7330)<br>< 0.80 > | 30 | LPRQ |
| 0133+476<br>J013658.59+475129.10 | BZQ | 0.859<br>0.859 | —<br>18.00<br>19.25 | <br>18.70<br>18.13 | **20.8 ± 0.7** [I90] | HPQ | 1986 | 14.6 ± 0.8 (6591)<br>6.4 ± 1.5 (7617)<br>4.1 ± 1.5 (7607)<br>< 8.75 > | 64 | HPQ |
| 0219+428<br>J022239.61+430207.80 | BZB | 0.370<br>0.370 | 15.71<br>15.21<br>14.50 | <br>—<br>— | 11.7 (med) [W92]<br>15.9 ± 0.7 (max) [M90]<br>15.5 ± 0.6 (max) [B90]<br>**(11 − 14) ± 0.4** [K76]<br>(6 − 15) [A80]<br>18.6 ± 0.8 (max) [S87]<br>18.7 ± 1.6 (max) [Si85] | HPQ | <br>1987<br>1987<br><br><br>1983<br>1982 | 11.9 ± 0.5 (6586)<br>6.5 ± 0.4 (6591)<br>6.0 ± 0.3 (6980)<br>< 7.99 > | 25 | HPQ |
| 0235+164<br>J023838.93+163659.27 | BZB | 0.940<br>0.940 | 16.46<br>15.50<br>15.92 | <br>—<br>— | 14.9 (med) [W92]<br>0.3 ± 0.1 [I90]<br>14.5 ± 3.7 (max) [M90]<br>15.4 ± 0.9 [F88]<br>15.5 ± 1.6 (max) [B90]<br>(6 − 25) [A80]<br>34.3 ± 3.3 (max) [S87]<br>8.0 ± 0.2 [W80]<br>13.3 ± 1.3 [W80]<br>**43.9 ± 1.4** [I82]<br>22.5 ± 1.8 (max) [Si85] | HPQ | <br>1976<br>1987<br>1984<br>1987<br><br>1984<br>1979<br>1979<br>1979<br>1982 | 22.0 ± 0.9 (6897)<br>17.6 ± 0.5 (6901)<br>10.8 ± 0.6 (6528)<br>< 12.15 > | 20 | HPQ |
| 0256+075<br>J025927.08+074739.64 | BZQ | 0.893<br>0.893 | 18.00<br>18.00<br>16.90 | <br>—<br>— | **16.0 ± 0.8** [K90]<br>9.5 ± 0.8 [K90] | HPQ | 1983<br>1984 | 36.3 ± 1.0 (7332)<br>35.1 ± 0.7 (7330)<br>23.2 ± 0.6 (6546)<br>< 23.59 > | 34 | HPQ |
| 0300+470<br>J030335.24+471616.28 | BZB | 0.475<br>0.475 | 17.54<br>16.95<br>16.20 | <br>—<br>— | 10.5 (med) [W92]<br>5.1 ± 4.9 [M90]<br>9.4 ± 1.5 (max) [B90]<br>(12 − 24) [A80]<br>**10.5 ± 0.9** [W80] | HPQ | <br>1987<br>1987<br><br>1980 | 8.8 ± 0.7 (6946)<br>4.5 ± 0.4 (6606)<br>3.7 ± 0.5 (6979)<br>< 7.25 > | 15 | HPQ |
| 0301-243<br>J030326.49-240711.50 | BZB | 0.266<br>0.266 | 16.55<br>16.18<br>— | <br>—<br>— | **10.6 ± 0.2** [I88] | HPQ | 1985 | 8.6 ± 0.4 (7262)<br>8.1 ± 0.4 (7332)<br>5.5 ± 0.4 (6600)<br>< 6.67 > | 12 | HPQ |
| 0316+413<br>J031948.20+413042.10 | BZU | 0.018<br>0.018 | 13.10<br>12.48<br>11.09 | <br>—<br>— | 0.6 ± 0.1 [I91]<br>(1 − 6) [A80]<br>3.5 ± 0.1 [M83]<br>0.9 ± 0.1 [A84] | HPQ | 1986<br><br>1976 | 1.2 ± 0.3 (6525)<br>− − −<br>− − −<br>< 1.20 > | 1 | LPRQ |
| 0317+185<br>J031951.80+184534.40 | BZG | 0.190<br>0.190 | —<br>18.12<br>— | <br>19.22<br>18.07 | **5.2 ± 0.8** (max) [J93] | HPQ | 1988 | 3.5 ± 0.6 (6605)<br>2.4 ± 0.4 (7336)<br>0.3 ± 0.6 (6885)<br>< 2.66 > | 7 | HPQ |
| 0333+321<br>J033630.11+321829.34 | BZQ | 1.258<br>1.263 | —<br>17.50<br>16.60 | <br>—<br>— | 0.8 (med) [W92]<br>0.7 ± 0.5 [W92]<br>1.0 ± 0.3 [M84]<br>0.9 ± 0.4 [M84]<br>1.6 ± 1.4 [M84]<br>0.5 ± 0.3 [M84]<br>0.1 ± 0.7 [M84] | LPRQ | <br>1985<br>1978<br>1979<br>1980<br>1980<br>1982 | 2.5 ± 0.5 (6912)<br>1.0 ± 0.4 (6979)<br>0.4 ± 0.5 (6946)<br>< 1.29 > | 7 | LPRQ |

*Continued on next page*

Table 1 – *Continued from previous page*

| Source SDSS name (1) | class (2) | z (3) | App. mag. (SIMBAD) B V R (4) | App. mag. (SDSS) g r (5) | $p_{opt}$ (%) (6) | Pol. class (7) | Epoch (8) | $p_{opt}$ (%) RoboPol p1 (JD*) p2 (JD*) p3 (JD*) mean p (9) | N (10) | Pol. class (RoboPol) (11) |
|---|---|---|---|---|---|---|---|---|---|---|
| 0336-019 | BZQ | 0.852 | 18.96 | | 11.8 (med)[W92] | HPQ | | 17.5 ± 1.5 (6601) | 4 | HPQ |
| J033930.94-014635.80 | | 0.852 | 18.41 | — | **19.4 ± 2.4** (max)[M81] | | 1979 | 8.7 ± 1.5 (6623) | | |
| | | | 17.33 | — | 8.6 ± 0.5[S88] | | 1986 | 7.1 ± 1.4 (6595) | | |
| | | | | | | | | < 9.78 > | | |
| 0338-214 | BZB | 0.223 | 16.04 | | **15.6 ± 2.9**[M90] | HPQ | 1987 | 5.2 ± 0.6 (6596) | 1 | HPQ |
| J034035.61-211931.17 | | 0.223 | 17.10 | — | 11.1 ± 1.6 (max)[B90] | | 1987 | – – – | | |
| | | | 17.07 | — | | | | – – – | | |
| | | | | | | | | < 5.20 > | | |
| 0403-132 | BZQ | 0.571 | 17.37 | | (0 – 4)[A80] | HPQ | | 1.7 ± 0.5 (6951) | 22 | LPRQ |
| J040534.00-130813.70 | | 0.571 | 17.09 | — | 3.9 ± 0.6 (max)[M81] | | 1978 | 1.6 ± 0.8 (7285) | | |
| | | | 16.60 | — | 1.4 ± 0.7[M84] | | 1980 | 1.1 ± 0.4 (7332) | | |
| | | | | | 3.8 ± 0.5[I90] | | 1985 | < 1.61 > | | |
| | | | | | 1.21 (med)[W92] | | | | | |
| 0414+009 | BZB | 0.287 | 16.86 | | 0.1 ± 0.7[M84] | HPQ | 1982 | 8.5 ± 0.4 (7264) | 4 | HPQ |
| J041652.49+010523.90 | | 0.287 | 16.38 | 17.24 | **5.1 ± 1.4** (max)[M90] | | 1988 | 5.5 ± 0.4 (7337) | | |
| | | | 16.00 | 16.87 | 7.8 ± 2.3 (max)[B90] | | 1987-88 | 4.8 ± 0.9 (6941) | | |
| | | | | | 2.8 ± 0.3[I88] | | 1985 | < 6.28 > | | |
| 0420-014 | BZQ | 0.916 | 17.50 | | 17.7 (med)[W92] | HPQ | | 27.9 ± 3.5 (7265) | 21 | HPQ |
| J042315.80-012033.06 | | 0.916 | 17.00 | — | (8 – 20)[A80] | | | 10.3 ± 2.7 (7331) | | |
| | | | 16.28 | — | 9.8 ± 1.2[F88] | | 1984 | 5.2 ± 2.0 (7332) | | |
| | | | | | 11.9 ± 0.5[I90] | | 1985 | < 10.00 > | | |
| | | | | | **20.2 ± 1.3** (max)[M81] | | 1978 | | | |
| | | | | | 8.5 ± 0.9[B86] | | 1984 | | | |
| | | | | | 16.1 ± 0.7 (max)[S88] | | 1986 | | | |
| 0440-003 | BZQ | 0.844 | 19.59 | | 1.7 (med)[W92] | HPQ | | 13.1 ± 1.9 (6525) | 15 | HPQ |
| J044238.66-001743.42 | | 0.844 | 19.22 | 18.42 | 2.7 ± 1.6[M84] | | 1980 | 6.4 ± 1.3 (6572) | | |
| | | | 17.85 | 18.16 | 0.7 ± 2.4[M84] | | 1980 | 4.7 ± 1.1 (6573) | | |
| | | | | | **12.6 ± 1.4**[F88] | | 1984 | < 6.32 > | | |
| 0716+714 | BZB | 0.310 | 15.50 | | 12.5 (med)[W92] | HPQ | | 11.5 ± 0.6 (6921) | 57 | HPQ |
| J072153.45+712036.36 | | 0.310 | 14.17 | — | **13.9 ± 1.2**[K90] | | 1979 | 9.3 ± 0.3 (7311) | | |
| | | | 14.27 | — | 28.6 ± 0.3[Bi81] | | 1980 | 5.8 ± 0.3 (6590) | | |
| | | | | | | | | < 11.37 > | | |
| 0735+178 | BZB | 0.450 | 16.76 | | 14.1 (med)[W92] | HPQ | | 11.6 ± 0.5 (6586) | 12 | HPQ |
| J073807.39+174219.00 | | 0.450 | 16.22 | 15.92 | 16.2 ± 0.5[I90] | | 1985 | 9.6 ± 0.5 (6778) | | |
| | | | 15.78 | 15.49 | 22.5 ± 1.0 (max)[M90] | | 1988 | 4.5 ± 0.6 (7335) | | |
| | | | | | 21.9 ± 1.0 (max)[B90] | | 1987-88 | < 7.70 > | | |
| | | | | | 18.4 ± 0.6[B86] | | 1982 | | | |
| | | | | | (4 – 31) ± 0.3[K76] | | | | | |
| | | | | | (3 – 31)[A80] | | | | | |
| | | | | | 31.9 ± 1.2 (max)[S87] | | 1984 | | | |
| | | | | | **36.9 ± 1.6**[P83] | | 1980 | | | |
| | | | | | 22.5 ± 0.3 (max)[Si85] | | 1982 | | | |
| 0748+126 | BZQ | 0.889 | 17.67 | | 1.4 (med)[W92] | (LPRQ) | | 12.3 ± 1.5 (6980) | 12 | HPQ |
| J075052.05+123104.83 | | 0.889 | 17.28 | 17.48 | 0.8 ± 1.2[W92] | | 1985 | 4.2 ± 1.1 (6780) | | |
| | | | 17.16 | 17.30 | **2.1 ± 1.1**[W92] | | 1986 | 1.9 ± 0.6 (6587) | | |
| | | | | | 1.0 ± 1.0[I90] | | 1984 | < 4.11 > | | |
| 0814+425 | BZB | 0.331 | 18.88 | | 3.9 ± 1.8[F88] | HPQ | 1984 | 17.0 ± 1.7 (6587) | 10 | HPQ |
| J081815.99+422245.41 | | 0.530 | 18.18 | 18.62 | 9.3 ± 0.9[W92] | | 1985 | 8.3 ± 3.5 (6804) | | |
| | | | 17.81 | 18.10 | 8.7 ± 1.4[I90] | | 1986 | 3.2 ± 0.8 (6979) | | |
| | | | | | **12.0 ± 0.6**[K90] | | 1984 | < 9.28 > | | |
| | | | | | 1.8 ± 0.5[K90] | | 1983 | | | |
| 0827+243 | BZQ | 0.939 | 17.62 | | 0.8 (med)[W92] | LPRQ | | 4.0 ± 0.5 (6774) | 13 | HPQ |
| J083052.09+241059.82 | | 0.941 | 17.26 | 17.37 | 0.1 ± 0.6[M84] | | 1979 | 1.6 ± 0.7 (6586) | | |
| | | | 16.30 | 17.12 | **1.5 ± 0.8**[M84] | | 1980 | 0.4 ± 0.3 (7152) | | |
| | | | | | | | | < 1.58 > | | |
| 0833+585 | BZQ | 2.103 | — | | 1.3 (med)[W92] | LPRQ | | 2.5 ± 0.5 (6595) | 2 | LPRQ |
| J083722.40+582501.80 | | 2.101 | 18.00 | 18.06 | 1.3 ± 0.9[W92] | | 1986 | 1.8 ± 0.5 (6605) | | |
| | | | 17.97 | 17.85 | | | | – – – | | |
| | | | | | | | | < 2.15 > | | |

*Continued on next page*

Table 1 – *Continued from previous page*

| Source<br>SDSS name<br><br><br><br><br>(1) | class<br><br><br><br><br><br>(2) | $z$<br><br><br><br><br><br>(3) | App. mag.<br>(SIMBAD)<br>B<br>V<br>R<br><br>(4) | App. mag.<br>(SDSS)<br><br>g<br>r<br><br>(5) | $p_{opt}$<br>(%)<br><br><br><br><br>(6) | Pol.<br>class<br><br><br><br><br>(7) | Epoch<br><br><br><br><br><br>(8) | $p_{opt}$ (%)<br>RoboPol<br>$p1$ (JD*)<br>$p2$ (JD*)<br>$p3$ (JD*)<br>mean $p$<br>(9) | N<br><br><br><br><br><br>(10) | Pol.<br>class<br>(RoboPol)<br><br><br><br>(11) |
|---|---|---|---|---|---|---|---|---|---|---|
| 0836+710<br>J084124.36+705342.17 | BZQ | 2.172<br>2.172 | —<br>16.50<br>16.80 | <br>—<br>— | 1.1 ± 0.5[I90]<br>1.0 ± 0.5[I91] | LPRQ | 1986<br>1986 | 2.6 ± 0.5 (6780)<br>0.7 ± 0.8 (7346)<br>0.6 ± 0.9 (7331)<br>< 2.55 > | 29 | LPRQ |
| 0846+513<br>J084957.98+510829.02 | BZU | 0.584<br>0.585 | 19.37<br>18.78<br>17.79 | <br>18.91<br>18.28 | 12.9 ± 3.2[M81]<br>**22.0 ± 2.3** (max)[Si85] | HPQ | 1980<br>1982 | 30.4 ± 1.5 (6799)<br>16.7 ± 2.0 (6803)<br>4.2 ± 0.9 (6580)<br>< 17.94 > | 5 | HPQ |
| 0850+581<br>J085442.00+575729.90 | BZQ | 1.317<br>1.319 | 18.56<br>18.18<br>17.43 | <br>18.15<br>17.74 | **0.4 ± 0.2**[I91] | LPRQ | 1986 | 9.4 ± 2.4 (6595)<br>3.8 ± 0.5 (7350)<br>0.8 ± 0.7 (7153)<br>< 3.44 > | 12 | HPQ |
| 0851+202<br>J085448.87+200630.64 | BZB | 0.306<br>0.306 | 15.91<br>15.43<br>15.56 | <br>15.93<br>15.42 | 12.5 (med)[W92]<br>14.5 ± 0.3[W92]<br>37.2 ± 0.4 (max)[S87]<br>(1 − 32)[A80]<br>10.8 ± 0.3[I90]<br>18.4 ± 0.7 (max)[M90]<br>18.4 ± 1.2[B90]<br>8.5 ± 0.5[B86]<br>(1 − 29) ± 0.2[K76]<br>**28.6 ± 0.3** (max)[Si85] | HPQ | <br>1987<br>1984<br><br>1985<br>1988<br>1988<br>1982<br><br>1983 | 14.8 ± 0.5 (6804)<br>10.4 ± 0.4 (6576)<br>5.8 ± 0.4 (7151)<br>< 12.35 > | 39 | HPQ |
| 0953+254<br>J095649.90+251516.10 | BZQ | 0.708<br>0.707 | 17.46<br>17.21<br>17.96 | <br>17.94<br>17.93 | 0.7 ± 0.4[M84]<br>2.2 ± 0.8[M84]<br>1.1 ± 1.1[W92]<br>1.5 ± 0.3[W92]<br>1.3 (med)[W92] | LPRQ | 1978<br>1980<br>1986<br>1987 | 2.4 ± 1.3 (6454)<br>− − −<br>− − −<br>< 2.40 > | 1 | (LPRQ) |
| 0954+556<br>J095738.18+552257.77 | BZQ | 0.901<br>0.900 | 18.24<br>17.89<br>— | <br>17.90<br>17.58 | 8.7 ± 0.8[W92]<br>**9.6 ± 1.8**[I90]<br>6.4 ± 0.5[I91] | HPQ | 1987<br>1976<br>1986 | 5.2 ± 0.6 (6828)<br>4.9 ± 0.5 (7350)<br>2.6 ± 0.9 (6466)<br>< 4.57 > | 13 | HPQ |
| 0954+658<br>J095847.24+653354.82 | BZB | 0.368<br>0.368 | —<br>17.00<br>15.75 | <br>—<br>— | 22.5 ± 0.6[W92]<br>19.1 ± 0.2[I91]<br>**33.7 ± 0.7**[K90] | HPQ | 1987<br>1986<br>1981 | 16.2 ± 0.5 (6831)<br>9.4 ± 0.3 (7331)<br>4.7 ± 0.5 (7333)<br>< 13.68 > | 19 | HPQ |
| 1012+232<br>J101447.10+230116.60 | BZQ | 0.566<br>0.566 | 17.85<br>17.78<br>16.22 | <br>17.39<br>17.52 | 0.7 (med)[W92]<br>**0.7 ± 0.6**[W92] | LPRQ | <br>1985 | 9.6 ± 8.2 (6452)<br>0.4 ± 0.6 (6455)<br>− − −<br>< 5.00 > | 2 | (HPQ) |
| 1038+064<br>J104117.20+061016.90 | BZQ | 1.271<br>1.265 | 16.86<br>16.70<br>16.14 | <br>17.05<br>16.92 | 0.6 (med)[W92]<br>0.6 ± 0.2[S84] | LPRQ | <br>1978 | 0.8 ± 0.6 (6452)<br>− − −<br>− − −<br>< 0.80 > | 1 | LPRQ |
| 1055+018<br>J105829.60+013358.80 | BZU | 0.894<br>0.890 | 18.74<br>18.28<br>16.68 | <br>18.30<br>17.85 | 4.9 ± 0.5[I88]<br>**5.0 ± 0.5**[I90]<br>4.4 ± 0.6[W92]<br>4.4 (med)[W92] | HPQ | 1984<br>1984<br>1985 | 9.5 ± 1.7 (6452)<br>− − −<br>− − −<br>< 9.50 > | 1 | HPQ |
| 1101+384<br>J110427.31+381231.80 | BZB | 0.030<br>0.029 | 13.50<br>12.90<br>8.31 | <br>13.60<br>13.08 | 3.8 ± 0.1 [M90]<br>3.7 ± 0.1 (max)[B90]<br>(0 − 6) ± 0.1[K76]<br>(0 − 7)[A80]<br>4.51 ± 0.06[W80]<br>**4.42 ± 0.04**[W80]<br>3.33 ± 0.09[W80]<br>3.76 ± 0.04[W80]<br>5.5 ± 0.4[Si85] | HPQ | 1988<br>1988<br><br><br>1980<br>1980<br>1980<br>1980<br>1982 | 5.8 ± 0.2 (6605)<br>− − −<br>− − −<br>< 5.80 > | 1 | HPQ |
| 1133+704<br>J113626.41+700927.31 | BZB | 0.045<br>0.045 | 15.16<br>14.49<br>10.51 | <br>—<br>— | **(1 − 4)**[A80] | HPQ | | 4.3 ± 0.3 (6831)<br>2.8 ± 0.3 (6588)<br>2.6 ± 0.4 (6808)<br>< 2.69 > | 18 | HPQ |

*Continued on next page*

Table 1 – *Continued from previous page*

| Source SDSS name (1) | class (2) | z (3) | App. mag. (SIMBAD) B V R (4) | App. mag. (SDSS) g r (5) | $p_{opt}$ (%) (6) | Pol. class (7) | Epoch (8) | $p_{opt}$ (%) RoboPol $p1$ (JD*) $p2$ (JD*) $p3$ (JD*) mean $p$ (9) | N (10) | Pol. class (RoboPol) (11) |
|---|---|---|---|---|---|---|---|---|---|---|
| 1156+295 | BZQ | 0.725 | 14.80 | | 9.2 (med)$^{W92}$ | HPQ | | 18.5 ± 0.9 (6467) | 2 | HPQ |
| J115931.83+291443.83 | | 0.725 | 14.41 | 18.22 | 2.7 ± 0.4$^{W92}$ | | 1987 | 5.7 ± 0.3 (6798) | | |
| | | | 17.65 | 18.09 | 29.8 ± 1.0 (max)$^{S87}$ | | 1983 | − − − | | |
| | | | | | (0.9 − 14.4)$^{S84}$ | | 1978-80 | < 12.10 > | | |
| | | | | | 24.8 ± 1.7 (max)$^{M90}$ | | 1988 | | | |
| | | | | | 27.3 ± 2.1 (max)$^{B90}$ | | 1988 | | | |
| | | | | | **14.4 ± 0.4** (max)$^{M81}$ | | 1980 | | | |
| | | | | | (1 − 9)$^{A80}$ | | | | | |
| | | | | | 27.1 ± 1.8 (max)$^{Si85}$ | | 1982 | | | |
| | | | | | 7.7 ± 0.7$^{S88}$ | | 1986 | | | |
| 1215+303 | BZB | 0.129 | 16.07 | | 8.0 (med)$^{W92}$ | HPQ | | 11.7 ± 0.4 (6858) | 16 | HPQ |
| J121752.08+300700.63 | | 0.130 | 15.62 | 15.56 | (5 − 14) ± 0.3$^{K76}$ | | | 11.2 ± 0.4 (6830) | | |
| | | | 13.47 | 15.24 | (4 − 17)$^{A80}$ | | | 8.1 ± 0.3 (6774) | | |
| | | | | | **16.2 ± 1.4**$^{Si85}$ | | 1982 | < 10.04 > | | |
| 1217+023 | BZQ | 0.240 | 16.15 | | 0.2 ± 0.3$^{S84}$ | LPRQ | 1978 | 1.1 ± 0.2 (6467) | 1 | LPRQ |
| J122011.90+020342.20 | | 0.240 | 15.97 | 15.84 | 0.2 (med)$^{W92}$ | | | − − − | | |
| | | | 15.60 | 15.82 | | | | − − − | | |
| | | | | | | | | < 1.10 > | | |
| 1219+285 | BZB | 0.102$^{a}$ | 16.81 | | 4.3 (med)$^{W92}$ | HPQ | | 16.1 ± 0.9 (6847) | 9 | HPQ |
| J122131.69+281358.50 | | 0.103 | 16.11 | 15.37 | **(2 − 10) ± 0.4**$^{K76}$ | | | 13.2 ± 0.8 (6443) | | |
| | | | 14.24 | 15.03 | (2 − 10)$^{A80}$ | | | 7.6 ± 0.4 (7184) | | |
| | | | | | | | | < 14.58 > | | |
| 1218+304 | BZB | 0.184 | 16.50 | | 6.6 (med)$^{W92}$ | HPQ | | 5.4 ± 0.7 (6830) | 7 | HPQ |
| J122121.94+301037.11 | | 0.182 | 15.85 | 16.26 | **6.6 ± 0.4**$^{W80}$ | | 1980 | 4.2 ± 1.3 (6793) | | |
| | | | 15.70 | 15.99 | 4.6 ± 0.2$^{W80}$ | | 1980 | 1.9 ± 0.4 (6866) | | |
| | | | | | 5.2 ± 0.2$^{W80}$ | | 1980 | < 3.07 > | | |
| | | | | | 6.8 ± 0.7 (max)$^{J93}$ | | 1990 | | | |
| | | | | | 8.4 ± 1.3$^{Si85}$ | | 1982 | | | |
| 1226+023 | BZQ | 0.158 | 13.05 | | 0.28 (med)$^{W92}$ | LPRQ | | 0.3 ± 0.1 (6450) | 1 | LPRQ |
| J122906.69+020308.59 | | 0.158 | 14.83 | 13.00 | 0.28 ± 0.09$^{W92}$ | | 1987 | − − − | | |
| | | | 14.11 | 12.89 | 0.37 ± 0.08$^{W92}$ | | 1987 | − − − | | |
| | | | | | 0.26 ± 0.11$^{W92}$ | | 1987 | < 0.30 > | | |
| | | | | | 0.21 ± 0.04$^{S84}$ | | 1978 | | | |
| | | | | | 0.31 ± 0.07$^{S84}$ | | 1978 | | | |
| | | | | | 0.39 ± 0.09$^{S84}$ | | 1978 | | | |
| | | | | | 0.20 ± 0.07$^{S84}$ | | 1978 | | | |
| | | | | | 0.31 ± 0.13$^{S84}$ | | 1978 | | | |
| | | | | | 0.25 ± 0.04$^{S84}$ | | 1980 | | | |
| | | | | | 0.5 ± 0.1$^{I90}$ | | 1984 | | | |
| | | | | | 0.4 ± 0.2 (max)$^{S87}$ | | 1984 | | | |
| | | | | | 0.8 ± 0.1$^{W80}$ | | 1980 | | | |
| | | | | | 0.3 ± 0.1$^{W80}$ | | 1980 | | | |
| | | | | | 2.5 ± 0.2$^{C88}$ | | 1988 | | | |
| 1253-055 | BZQ | 0.536 | 18.01 | | 8.6 (med)$^{W92}$ | HPQ | | 23.5 ± 0.4 (6467) | 20 | HPQ |
| J125611.17-054721.52 | | 0.536 | 17.75 | — | 11.4 ± 5.3 (max)$^{S87}$ | | 1983 | 21.0 ± 0.4 (6808) | | |
| | | | 15.87 | — | (4 − 19)$^{A80}$ | | | 18.4 ± 0.5 (6804) | | |
| | | | | | 9.0 ± 0.4$^{I90}$ | | 1985 | < 18.71 > | | |
| | | | | | 44.3 ± 1.0 (max)$^{M90}$ | | 1986 | | | |
| | | | | | 41.6 ± 0.6 (max)$^{B90}$ | | 1986-88 | | | |
| | | | | | **11.8 ± 0.3** (max)$^{M81}$ | | 1979 | | | |
| | | | | | 9.8 ± 1.1$^{Si85}$ | | 1983 | | | |
| 1334-127 | BZQ | 0.539 | 18.50 | | **16.1 ± 0.3**$^{K90}$ | HPQ | 1985 | 8.6 ± 1.7 (6465) | 1 | HPQ |
| J133739.78-125724.69 | | 0.539 | 18.50 | — | 10.6 ± 0.5$^{I90}$ | | 1984 | − − − | | |
| | | | 16.22 | — | | | | − − − | | |
| | | | | | | | | < 8.60 > | | |
| 1418+546 | BZB | 0.153 | 16.17 | | (2 − 19)$^{A80}$ | HPQ | | 4.3 ± 0.2 (6466) | 1 | HPQ |
| J141946.60+542314.80 | | 0.153 | 15.65 | 15.83 | **11.9 ± 0.3**$^{W80}$ | | 1980 | − − − | | |
| | | | 14.16 | 15.38 | 13.0 ± 3.0$^{P83}$ | | 1980 | − − − | | |
| | | | | | 16.9 ± 1.5 (max)$^{Si85}$ | | 1982 | < 4.30 > | | |
| | | | | | 17.0 ± 0.5 (max)$^{S87}$ | | 1983 | | | |
| | | | | | 17.5 ± 4.8 (max)$^{M90}$ | | 1987 | | | |
| | | | | | 15.4 ± 2.8 (max)$^{B90}$ | | 1986-88 | | | |

*Continued on next page*

Table 1 – *Continued from previous page*

| Source<br>SDSS name<br><br>(1) | class<br><br>(2) | $z$<br><br>(3) | App. mag.<br>(SIMBAD)<br>B<br>V<br>R<br>(4) | App. mag.<br>(SDSS)<br>g<br>r<br>(5) | $p_{opt}$<br>(%)<br><br>(6) | Pol.<br>class<br><br>(7) | Epoch<br><br>(8) | $p_{opt}$ (%)<br>RoboPol<br>$p1$ (JD*)<br>$p2$ (JD*)<br>$p3$ (JD*)<br>mean $p$<br>(9) | N<br><br>(10) | Pol.<br>class<br>(RoboPol)<br>(11) |
|---|---|---|---|---|---|---|---|---|---|---|
| | | | | | 7.5 (med) [W92] | | | | | |
| 1424+240<br>J142700.39+234800.04 | BZB | 0.604<br>0.604 | 14.34<br>14.95<br>14.50 | 14.88<br>14.57 | **$4.7 \pm 0.3$** [I88]<br>$5.1 \pm 0.6$ (max) [B90]<br>$5.0 \pm 0.5$ (max) [M90]<br>$4.5 \pm 0.4$ [I88] | HPQ | 1984<br>1988<br>1988<br>1985 | $7.2 \pm 0.4$ (7264)<br>$5.6 \pm 0.2$ (6455)<br>$4.0 \pm 0.3$ (6872)<br>$< 5.54 >$ | 12 | HPQ |
| 1426+428<br>J142832.66+424020.60 | BZB | 0.129<br>0.129 | 16.95<br>16.45<br>14.40 | 16.75<br>16.14 | $2.5 \pm 0.6$ [J93]<br>$2.4 \pm 0.3$ [J93] | (LPRQ) | 1989<br>1989 | $2.8 \pm 0.4$ (6872)<br>$2.3 \pm 0.4$ (6822)<br>$2.1 \pm 0.4$ (6885)<br>$< 1.85 >$ | 13 | LPRQ |
| 1435+638<br>J143645.80+633637.90 | BZQ | 2.066<br>2.066 | 17.06<br>16.86<br>16.23 | 17.06<br>16.98 | 0.3 (med) [W92]<br>$0.3 \pm 0.5$ [W92] | LPRQ | <br>1986 | $1.6 \pm 0.3$ (6469)<br>– – –<br>– – –<br>$< 1.60 >$ | 1 | LPRQ |
| 1508-055<br>J151053.60-054307.40 | BZQ | 1.185<br>1.185 | 17.44<br>17.21<br>— | —<br>— | $1.5 \pm 0.5$ [S84]<br>$2.0 \pm 0.8$ [S84]<br>1.8 (med) [W92] | LPRQ | 1978<br>1980 | $2.0 \pm 0.6$ (6455)<br>– –<br>– – –<br>$< 2.00 >$ | 1 | LPRQ |
| 1510-089<br>J151250.53-090559.83 | BZQ | 0.361[b]<br>0.360 | 16.74<br>16.54<br>— | —<br>— | 2.4 (med) [W92]<br>$2.6 \pm 0.6$ [W92]<br>$8.9 \pm 3.0$ [S87]<br>$(1.2 - 7.8)$ [S84]<br>$0.7 \pm 0.9$ [S84]<br>$1.9 \pm 0.4$ [I90]<br>**$7.8 \pm 0.5$** (max) [M81]<br>$12.6 \pm 1.1$ [S88] | HPQ | <br>1985<br>1983<br>1978-80<br>1981<br>1978<br>1980<br>1987 | $5.6 \pm 0.5$ (7200)<br>$3.0 \pm 0.3$ (7188)<br>$2.1 \pm 0.5$ (7935)<br>$< 5.13 >$ | 98 | HPQ |
| 1514+197<br>J151656.79+193212.99 | BZB | 1.070<br>1.070 | 18.19<br>18.70<br>17.51 | 18.94<br>18.37 | 8.0 (med) [W92]<br>$(7 - 9) \pm 2.8$ [K76]<br>$(7 - 9)$ [A80] | HPQ | | $1.4 \pm 1.1$ (6450)<br>– – –<br>– – –<br>$< 1.40 >$ | 1 | LPRQ |
| 1514-241<br>J151741.80-242219.50 | BZB | 0.049<br>0.048 | 15.13<br>14.00<br>13.95 | —<br>— | **$(2 - 6) \pm 0.4$** [K76]<br>$4.9 \pm 0.6$ [B86]<br>$4.2 \pm 0.2$ [B86]<br>$4.8 \pm 0.3$ (max) [B90]<br>$4.8 \pm 0.3$ [M90]<br>5.7 (med) [W92] | HPQ | <br>1984<br>1984<br>1986-87<br>1987 | $3.1 \pm 0.4$ (6455)<br>– – –<br>– – –<br>$< 3.10 >$ | 1 | (HPQ) |
| 1548+056<br>J155035.30+052710.40 | BZQ | 1.420<br>1.422 | 19.10<br>18.73<br>19.02 | 18.63<br>18.27 | $4.6 \pm 1.1$ [I88]<br>$2.9 \pm 1.3$ [I88]<br>**$4.7 \pm 1.1$** [I90] | HPQ | 1984<br>1985<br>1984 | $6.5 \pm 2.3$ (6454)<br>$3.9 \pm 1.8$ (6470)<br>– – –<br>$< 5.20 >$ | 2 | HPQ |
| 1551+130<br>J155332.69+125651.72 | BZQ | 1.309<br>1.308 | 18.05<br>17.65<br>17.10 | 17.43<br>17.30 | **$0.7 \pm 1.0$** [W92] | LPRQ | 1986 | $3.3 \pm 0.7$ (6851)<br>$1.5 \pm 0.5$ (6823)<br>$0.2 \pm 0.4$ (6486)<br>$< 1.83 >$ | 47 | HPQ |
| 1606+105<br>J160846.20+102907.80 | BZQ | 1.233<br>1.226 | 18.50<br>18.00<br>18.03 | 18.38<br>18.09 | $2.1 \pm 0.9$ [I90] | LPRQ | 1986 | $3.0 \pm 2.5$ (6444)<br>$0.8 \pm 1.1$ (6470)<br>$0.6 \pm 1.3$ (6455)<br>$< 1.47 >$ | 3 | (LPRQ) |
| 1633+382<br>J163515.49+380804.50 | BZQ | 1.814<br>1.813 | 18.14<br>17.97<br>17.25 | 17.66<br>17.62 | 1.1 (med) [W92]<br>$0.8 \pm 0.9$ [W92]<br>$1.1 \pm 0.2$ [I91]<br>$2.6 \pm 1.0$ [M84]<br>$1.4 \pm 1.1$ [M84]<br>**$0.5 \pm 0.7$** [M84] | (LPRQ) | <br>1986<br>1986<br>1980<br>1980<br>1981 | $7.8 \pm 0.4$ (7636)<br>$4.9 \pm 0.7$ (6882)<br>$2.3 \pm 0.4$ (7156)<br>$< 7.26 >$ | 99 | HPQ |
| 1637+574<br>J163813.46+572023.98 | BZQ | 0.751<br>0.751 | —<br>17.00<br>16.94 | —<br>— | 1.2 (med) [W92]<br>$1.5 \pm 0.7$ [W92]<br>$0.9 \pm 0.5$ [W92]<br>$2.4 \pm 0.8$ [I91] | (LPRQ) | <br>1986<br>1986<br>1986 | $1.0 \pm 1.0$ (7162)<br>$0.8 \pm 0.4$ (6521)<br>$0.1 \pm 0.3$ (6914)<br>$< 0.74 >$ | 40 | LPRQ |

*Continued on next page*

Table 1 – *Continued from previous page*

| Source<br>SDSS name<br><br><br><br><br>(1) | class<br><br><br><br><br><br>(2) | $z$<br><br><br><br><br><br>(3) | App. mag.<br>(SIMBAD)<br>B<br>V<br>R<br><br>(4) | App. mag.<br>(SDSS)<br><br>g<br>r<br><br>(5) | $p_{opt}$<br>(%)<br><br><br><br><br>(6) | Pol.<br>class<br><br><br><br><br>(7) | Epoch<br><br><br><br><br><br>(8) | $p_{opt}$ (%)<br>RoboPol<br>$p1$ (JD*)<br>$p2$ (JD*)<br>$p3$ (JD*)<br>mean $p$<br>(9) | N<br><br><br><br><br><br>(10) | Pol.<br>class<br>(RoboPol)<br><br><br><br>(11) |
|---|---|---|---|---|---|---|---|---|---|---|
| 1638+398<br>J164029.60+394646.00 | BZQ | 1.672<br>1.666 | 18.40<br>16.50<br>18.75 | <br>19.78<br>19.54 | 4.8 ± 1.2[K90]<br>**9.9 ± 2.0**[K90] | HPQ | 1985 | 5.3 ± 2.5 (6452)<br>– – –<br>– – –<br>< 5.30 > | 1 | (HPQ) |
| 1641+399<br>J164258.81+394836.99 | BZQ | 0.593<br>0.593 | 16.81<br>16.59<br>16.84 | <br>15.68<br>15.39 | 6.7 (med)[W92]<br>3.6 ± 0.2[S78]<br>(3.6 – 15.6)[S84]<br>12.3 ± 0.5[S84]<br>4.0 ± 0.3[I90]<br>11.2 ± 0.2[I91]<br>12.6 ± 0.8 (max)[M90]<br>16.1 ± 1.1 (max)[B90]<br>**15.6 ± 0.3** (max)[M81]<br>(2 – 16)[A80]<br>35.3 ± 0.9[S86]<br>28.7 ± 0.4 (max)[Si85] | HPQ | <br>1977<br>1977-80<br>1980<br>1973<br>1986<br>1986<br>1986-87<br>1978<br><br>1983<br>1983 | 15.0 ± 0.6 (7153)<br>9.8 ± 4.0 (6509)<br>3.7 ± 0.9 (7174)<br>< 5.54 > | 44 | HPQ |
| 1652+398<br>J165352.22+394536.61 | BZB | 0.033<br>0.034 | 14.15<br>13.29<br>8.26 | <br>14.37<br>13.28 | 3.0 ± 0.1[I91]<br>2.5 ± 0.2[M90]<br>(2 – 4)[A80]<br>1.6 ± 0.2 (max)[B90]<br>3.0 ± 0.5[B86]<br>(2 – 3) ± 0.2[K76]<br>4.2 ± 0.2 (max)[J93]<br>3.6 ± 0.1[A84] | HPQ | 1986<br>1987<br><br>1987<br>1982<br><br>1989 | 3.0 ± 0.3 (6550)<br>2.5 ± 0.2 (6863)<br>2.0 ± 0.3 (6528)<br>< 2.29 > | 73 | LPRQ |
| 1722+119<br>J172504.34+115215.47 | BZB | 0.018<br>0.018 | 16.29<br>15.77<br>14.45 | <br>—<br>— | **15.5 ± 0.4** (max)[J93] | HPQ | 1989 | 7.5 ± 0.4 (6495)<br>5.4 ± 0.3 (7238)<br>4.3 ± 0.4 (7223)<br>< 7.19 > | 89 | HPQ |
| 1727+502<br>J172818.62+501310.47 | BZB | 0.055<br>0.055 | 16.55<br>15.97<br>12.95 | <br>—<br>— | 5.0 (med)[W92]<br>1.1 ± 1.9 [M90]<br>2.5 ± 0.8 (max)[B90]<br>**(4 – 6) ± 0.4**[K76]<br>(4 – 6)[A80] | HPQ | <br>1987<br>1987 | 3.4 ± 0.3 (7264)<br>2.4 ± 0.4 (6882)<br>1.2 ± 0.3 (6778)<br>< 2.27 > | 13 | HPQ |
| 1749+701<br>J174832.84+700550.77 | BZB | 0.770<br>0.770 | 17.46<br>17.01<br>15.48 | <br>—<br>— | 11.5 (med)[W92]<br>19.1 ± 0.3[W92]<br>20.3 ± 0.3[W92]<br>10.5 ± 0.2[I91]<br>8.9 ± 0.4[K90]<br>**11.5 ± 0.3**[W80]<br>5.9 ± 0.4[W80]<br>3.5 ± 0.4[W80] | HPQ | <br>1986<br>1986<br>1986<br>1985<br>1980<br>1980<br>1980 | 12.7 ± 0.4 (7224)<br>8.9 ± 0.5 (7193)<br>8.5 ± 0.4 (6524)<br>< 10.31 > | 94 | HPQ |
| 1749+096<br>J175132.82+093900.73 | BZB | 0.322<br>0.320 | 17.46<br>16.78<br>15.57 | <br>—<br>— | 9.0 (med)[W92]<br>**23.1 ± 5.0**[S87]<br>6.0 ± 1.8[I90]<br>19.0 ± 6.8 [M90]<br>16.5 ± 1.0 (max)[B90]<br>31.3 ± 0.6 (max)[B86]<br>(3 – 9) ± 1.8[K76]<br>(3 – 9)[A80] | HPQ | <br>1983<br><br>1987<br>1987<br>1984 | 16.6 ± 0.7 (6881)<br>8.8 ± 0.5 (7239)<br>5.6 ± 0.4 (7265)<br>< 10.28 > | 96 | HPQ |
| 1803+784<br>J180045.68+782804.02 | BZB | 0.680<br>0.684 | 16.40<br>16.40<br>15.46 | <br>17.46<br>17.10 | 35.2 (med)[W92]<br>7.0 ± 0.2[I91]<br>**35.2 ± 0.4**[Bi81] | HPQ | <br>1986<br>1979 | 9.2 ± 0.3 (6542)<br>6.7 ± 0.5 (7597)<br>6.7 ± 0.4 (7601)<br>< 8.07 > | 79 | HPQ |
| 1807+698<br>J180650.68+694928.11 | BZB | 0.049<br>0.051 | 14.77<br>14.22<br>11.39 | <br>—<br>— | 8.0 ± 0.1[I91]<br>(0 – 12)[A80]<br>**(0 – 12) ± 0.2**[K76]<br>10.1 ± 0.2 (max)[M75] | HPQ | 1986<br><br><br>1974 | 6.3 ± 0.4 (7234)<br>5.6 ± 0.3 (7262)<br>5.0 ± 0.3 (6518)<br>< 5.40 > | 84 | HPQ |
| 1823+568<br>J182407.07+565101.49 | BZB | 0.664<br>0.664 | 18.90<br>18.40<br>16.48 | <br>—<br>— | 16.8 ± 0.7[I90]<br>2.6 ± 0.8[K90]<br>9.4 ± 2.4[K90]<br>**11.5 ± 2.2**[K90] | HPQ | 1986<br>1982<br>1981<br>1981 | 3.4 ± 0.3 (6453)<br>1.3 ± 1.0 (6444)<br>– – –<br>< 2.35 > | 2 | HPQ |

*Continued on next page*

Table 1 – *Continued from previous page*

| Source<br>SDSS name<br>(1) | class<br>(2) | $z$<br>(3) | App. mag.<br>(SIMBAD)<br>B<br>V<br>R<br>(4) | App. mag.<br>(SDSS)<br>g<br>r<br>(5) | $p_{opt}$<br>(%)<br>(6) | Pol.<br>class<br>(7) | Epoch<br>(8) | $p_{opt}$ (%)<br>RoboPol<br>$p1$ (JD*)<br>$p2$ (JD*)<br>$p3$ (JD*)<br>mean $p$<br>(9) | N<br>(10) | Pol.<br>class<br>(RoboPol)<br>(11) |
|---|---|---|---|---|---|---|---|---|---|---|
| 1926+611<br>J192730.44+611732.88 | BZB | —<br>0.540 | 17.50<br>17.50<br>16.99 | <br>17.57<br>17.18 | 9.7 (med)[W92]<br>9.3 ± 1.1[W92]<br>10.0 ± 0.7[W92]<br>**6.5 ± 0.7**[K90] | HPQ | <br>1985<br>1986<br>1984 | 13.2 ± 0.6 (6490)<br>8.1 ± 0.5 (7194)<br>7.3 ± 0.6 (7214)<br>< 8.28 > | 37 | HPQ |
| 1928+738<br>J192748.49+735801.57 | BZQ | 0.302<br>0.302 | —<br>15.50<br>15.11 | <br>—<br>— | 1.1 (med)[W92]<br>1.5 ± 0.4[W92]<br>0.8 ± 0.4[Bi81]<br>1.2 ± 0.1[I91] | LPRQ | <br>1985<br>1979<br>1986 | 2.0 ± 0.3 (6942)<br>1.8 ± 0.3 (7332)<br>1.7 ± 0.4 (7285)<br>< 1.72 > | 28 | LPRQ |
| 1954+513<br>J195542.74+513148.55 | BZQ | 1.220<br>1.230 | —<br>18.50<br>17.34 | <br>—<br>— | 1.5 (med)[W92]<br>**1.5 ± 0.5**[M84] | LPRQ | <br>1980 | 3.4 ± 0.5 (7214)<br>2.7 ± 0.5 (7252)<br>2.1 ± 0.5 (7224)<br>< 2.78 > | 17 | HPQ |
| 1958-179<br>J200057.09-174857.67 | BZQ | 0.652<br>0.650 | 18.02<br>17.46<br>15.33 | <br>—<br>— | 20.4 (med)[W92]<br>**25.3 ± 1.1**[W92]<br>19.4 ± 0.8[W92]<br>20.4 ± 0.7[W92]<br>22.7 ± 9.3[W92]<br>14.5 ± 0.2[S88] | HPQ | <br>1985<br>1986<br>1986<br>1986<br>1987 | 13.6 ± 1.6 (6452)<br>− − −<br>− − −<br>< 13.60 > | 1 | HPQ |
| 2007+777<br>J200530.93+775243.10 | BZB | 0.342<br>0.342 | —<br>16.50<br>17.36 | <br>16.72<br>16.16 | 15.1 (med)[W92]<br>**15.1 ± 0.9**[Bi81] | HPQ | <br>1979 | 11.9 ± 0.4 (7601)<br>4.5 ± 0.4 (6530)<br>2.8 ± 0.5 (7604)<br>< 6.00 > | 76 | HPQ |
| 2021+614<br>J202206.70+613658.80 | BZQ | 0.227<br>0.227 | —<br>19.50<br>17.58 | <br>—<br>— | **0.3 ± 0.3**[I91] | LPRQ | 1986 | 5.6 ± 1.6 (6588)<br>4.7 ± 1.3 (6541)<br>1.3 ± 1.2 (6593)<br>< 4.03 > | 7 | HPQ |
| 2023+760<br>J202235.58+761126.17 | BZB | 0.594<br>0.594 | —<br>18.10<br>17.54 | <br>17.32<br>16.68 | **13.6 ± 1.0**[K90] | HPQ | 1984 | 14.3 ± 0.5 (7604)<br>13.6 ± 0.4 (6524)<br>10.9 ± 0.4 (7609)<br>< 11.93 > | 72 | HPQ |
| 2032+107<br>J203522.30+105606.80 | BZQ | 0.601<br>0.601 | 17.96<br>16.37<br>17.40 | <br>—<br>— | 12.0[A80]<br>1.4 ± 1.1[M90]<br>12.2 (med)[W92] | HPQ | <br>1987 | 0.8 ± 2.3 (6454)<br>− − −<br>− − −<br>< 0.80 > | 1 | LPRQ |
| 2141+175<br>J214335.54+174348.79 | BZQ | 0.211<br>0.211 | 15.91<br>15.73<br>15.17 | <br>16.25<br>16.04 | 0.2 (med)[W92]<br>0.2 ± 0.2[S84] | LPRQ | <br>1977 | 1.4 ± 0.4 (6523)<br>1.4 ± 0.3 (7603)<br>0.8 ± 0.4 (7598)<br>< 1.14 > | 76 | LPRQ |
| 2145+067<br>J214805.46+065738.60 | BZQ | 1.003<br>0.999 | 16.85<br>16.47<br>15.06 | <br>16.12<br>15.88 | 0.9 (med)[W92]<br>0.9 ± 0.8[W92]<br>1.0 ± 0.4[W92]<br>**0.6 ± 0.2**[S84]<br>0.5 ± 0.4[S84]<br>0.3 ± 0.5[S84] | LPRQ | <br>1985<br>1986<br>1977<br>1977<br>1977 | 3.7 ± 0.6 (6510)<br>1.6 ± 1.2 (7609)<br>1.3 ± 0.8 (7604)<br>< 1.28 > | 70 | HPQ |
| 2150+173<br>J215224.80+173437.80 | BZB | 0.870<br>0.874 | —<br>17.90<br>17.98 | <br>19.56<br>18.98 | **25.7 ± 0.5**[K90] | HPQ | 1983 | 6.8 ± 4.3 (6462)<br>− − −<br>− − −<br>< 6.80 > | 1 | (HPQ) |
| 2200+420<br>J220243.29+421639.98 | BZB | 0.069<br>0.069 | 15.66<br>14.72<br>— | <br>—<br>— | 9.8 (med)[W92]<br>4.9 ± 0.4[I90]<br>**13.7 ± 0.1**[I91]<br>14.2 ± 0.5 (max)[M90]<br>14.2 ± 0.4 (max)[B90]<br>12.5 ± 1.9[B86]<br>(2 − 19) ± 0.3[K76]<br>(2 − 23)[A80]<br>18.9 ± 0.8 (max)[S87]<br>2.4 ± 0.3[W80]<br>18.9 ± 2.6[P83]<br>23.1 ± 3.1 (max)[Si85] | HPQ | <br>1978<br>1986<br>1986<br>1986-87<br>1982<br><br><br>1984<br>1980<br>1979<br>1982 | 9.0 ± 0.3 (6519)<br>5.9 ± 0.3 (7350)<br>3.9 ± 0.2 (7603)<br>< 6.61 > | 142 | HPQ |

*Continued on next page*

Table 1 – *Continued from previous page*

| Source SDSS name (1) | class (2) | $z$ (3) | App. mag. (SIMBAD) B V R (4) | App. mag. (SDSS) g r (5) | $p_{opt}$ (%) (6) | Pol. class (7) | Epoch (8) | $p_{opt}$ (%) RoboPol $p1$ (JD*) $p2$ (JD*) $p3$ (JD*) mean $p$ (9) | N (10) | Pol. class (RoboPol) (11) |
|---|---|---|---|---|---|---|---|---|---|---|
| 2223-052 | BZQ | 1.404 | 18.83 | | 8.8 (med) [W92] | HPQ | | $16.0 \pm 1.9$ (6882) | 33 | HPQ |
| J222547.26-045701.39 | | 1.404 | 18.39 | 18.04 | $2.4 \pm 0.6$ [W92] | | 1986 | $1.1 \pm 0.8$ (7336) | | |
| | | | 16.30 | 17.56 | $14.2 \pm 2.1$ (max) [S87] | | 1983 | $1.1 \pm 0.8$ (7337) | | |
| | | | | | **$13.6 \pm 0.4$** [S78] | | 1977 | $< 5.95 >$ | | |
| | | | | | $17.4 \pm 2.4$ (max) [M90] | | 1987 | | | |
| | | | | | $11.9 \pm 1.2$ (max) [B90] | | 1987 | | | |
| | | | | | $(10 - 17)$ (max) [M81] | | 1977 | | | |
| | | | | | $(4 - 17)$ [A80] | | | | | |
| | | | | | $11.2 \pm 1.5$ (max) [Si85] | | 1982 | | | |
| | | | | | $7.8 \pm 0.6$ [S88] | | 1986 | | | |
| 2227-088 | BZQ | 1.560 | 17.80 | | $6.6 \pm 5.3$ [I90] | HPQ | 1985 | $6.2 \pm 0.6$ (7966) | 7 | HPQ |
| J222940.10-083254.40 | | 1.561 | 17.41 | 17.43 | $2.3 \pm 1.2$ [W92] | | 1985 | $4.5 \pm 0.6$ (8046) | | |
| | | | 17.81 | 17.07 | $8.0 \pm 1.0$ [W92] | | 1985 | $2.2 \pm 0.7$ (8065) | | |
| | | | | | **$9.2 \pm 0.9$** [W92] | | 1985 | $< 4.36 >$ | | |
| | | | | | $5.8 \pm 1.3$ [W92] | | 1986 | | | |
| | | | | | 6.9 (med) [W92] | | | | | |
| 2230+114 | BZQ | 1.032 | 17.75 | | 7.3 (med) [W92] | HPQ | | $13.3 \pm 0.3$ (7630) | 110 | HPQ |
| J223236.41+114350.90 | | 1.037 | 17.33 | 17.09 | $(1 - 11)$ [A80] | | | $6.5 \pm 0.7$ (6947) | | |
| | | | — | 16.71 | $6.7 \pm 0.9$ [B86] | | 1984 | $3.2 \pm 0.4$ (8015) | | |
| | | | | | $7.3 \pm 0.3$ [I90] | | 1978 | $< 5.06 >$ | | |
| | | | | | **$10.9 \pm 0.4$** (max) [M81] | | 1978 | | | |
| 2251+158 | BZQ | 0.859 | 16.57 | | 3.1 (med) [W92] | HPQ | | $9.0 \pm 0.4$ (7262) | 164 | HPQ |
| J225357.75+160853.56 | | 0.859 | 16.10 | 15.60 | $1.4 \pm 0.5$ [W92] | | 1986 | $7.5 \pm 0.3$ (6951) | | |
| | | | 15.22 | 15.10 | **$9.3 \pm 2.3$** (max) [S87] | | 1983 | $5.3 \pm 0.4$ (6525) | | |
| | | | | | $(0.1 - 3.5)$ [S84] | | 1977-79 | $< 5.90 >$ | | |
| | | | | | $2.9 \pm 0.3$ [I90] | | 1978 | | | |
| | | | | | $3.7 \pm 1.1$ [M90] | | 1987 | | | |
| | | | | | $4.2 \pm 1.0$ (max) [B90] | | 1987 | | | |
| | | | | | $3.5 \pm 0.6$ (max) [M81] | | 1979 | | | |
| | | | | | $(0 - 16)$ [A80] | | | | | |
| | | | | | $0.4 \pm 0.4$ [S78] | | 1977 | | | |
| | | | | | $2.0 \pm 1.3$ [Si85] | | 1982 | | | |
| | | | | | $3.3 \pm 0.3$ (max) [S88] | | 1987 | | | |
| 2345-167 | BZQ | 0.576 | 18.00 | | $(3 - 19)$ [A80] | HPQ | | $18.5 \pm 0.9$ (6610) | 1 | HPQ |
| J234802.60-163112.00 | | 0.576 | 18.41 | — | **$18.5 \pm 1.7$** (max) [M81] | | 1979 | – – – | | |
| | | | 16.86 | — | $1.9 \pm 1.9$ [B86] | | 1984 | – – – | | |
| | | | | | $11.8 \pm 4.3$ [S88] | | 1986 | $< 18.50 >$ | | |
| | | | | | 4.0 (med) [W92] | | | | | |

Col. (2): The source class is taken from the 5th edition of ROMA-BZCAT (Massaro et al. 2015) where the BZB stands for BL Lac type of blazar, BZQ stands for FSRQ type blazar, BZG: BL Lac-galaxy dominated and BZU: blazars of Uncertain type;
Col. (3): Redshift, the upper value is from NED and the lower value is from Blinov et al. (2021). The redshift marked with 'a' or 'b' is taken from Tarnopolski et al. (2020) and Landoni et al. (2020) respectively;
Col. (6): The reference codes for polarization are available in the footnotes of Table 1 in the main manuscript;
Col. (7): polarization class of the source ($p_{opt}$ (max) $\leq 3\%$ for LPRQs and $> 3\%$ for HPQs). The polarization class in parentheses is for border-line cases for which the quoted one-$\sigma$ error on $p_{max}$ would push the source to the other polarization class;
Col. (8): Epoch of the $p_{opt}$ measurement;
Col. (9): RoboPol measured $p_{opt}$, taken from Blinov et al. (2021). The JD in parentheses marked with '*' corresponds to Julian date minus 2450000. The parameters $p1$, $p2$ and $p3$ are explained in section 2;
Col. (10): Number of RoboPol polarization measurements;
Col. (11): polarization class of the source ($p_{opt}$ (max) $\leq 3\%$ for LPRQs and $> 3\%$ for HPQs). The polarization class in parentheses is for those six sources for which the quoted one-$\sigma$ error on $p_{max}$ would push the source to the other polarization class. Note that all these six sources have the number of RoboPol measurements N $< 5$.

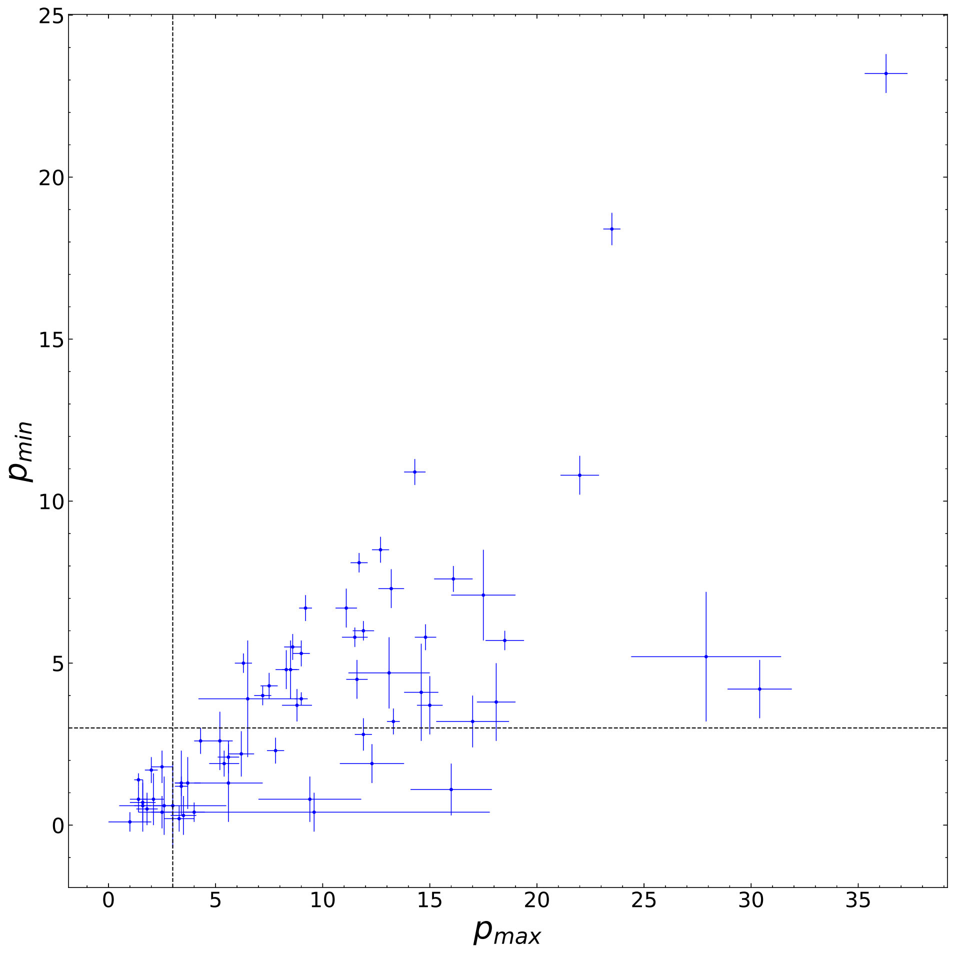


**Figure S1.** $p_{max}$ vs $p_{min}$ plot for the 64 sources covered in RoboPol survey, for which N > 1.

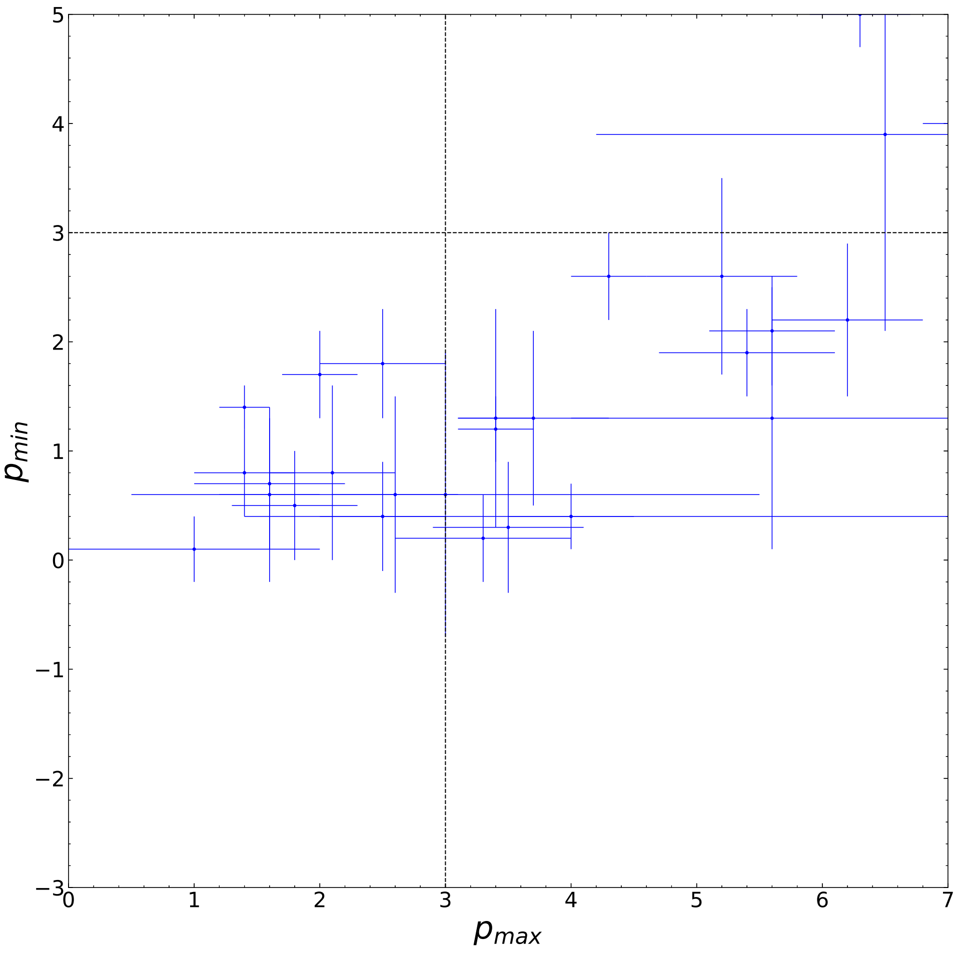


**Figure S2.** The zoomed version of Figure S1.

## REFERENCES

Blinov D., et al., 2021, MNRAS, 501, 3715
Landoni M., Falomo R., Paiano S., Treves A., 2020, ApJS, 250, 37
Massaro E., Maselli A., Leto C., Marchegiani P., Perri M., Giommi P., Piranomonte S., 2015, Ap&SS, 357, 75
Tarnopolski M., Żywucka N., Marchenko V., Pascual-Granado J., 2020, ApJS, 250, 1
